# Supplementary material for: Maximum entropy mediated liquid-to-solid nucleation and transition
Source: arXiv:2411.17348 ancillary file (2024-11-26)
Supplement: Supplementary file 1 [file SIAverageBondOrderParameters.pdf]

# Supporting Information: Maximum entropy mediated liquid-to-solid nucleation and transition

Lars Dammann*

*Hamburg University of Technology, Institute for Soft Matter Modeling & Institute for Materials and X-Ray Physics, Hamburg, DE 21073, Germany.*

*Deutsches Elektronen-Synchrotron DESY, Hamburg, DE 22607, Germany.*

Richard Kohns and Patrick Huber

*Hamburg University of Technology, Institute for Materials and X-Ray Physics, Hamburg, DE 21073, Germany.*

*Deutsches Elektronen-Synchrotron DESY, Hamburg, DE 22607, Germany.*

Robert H. Meißner*

*Hamburg University of Technology, Institute for Soft Matter Modeling, Hamburg, DE 21073, Germany*

*Helmholtz-Zentrum Hereon, Institute of Surface Science, Geesthacht, DE 21502, Germany*

(Dated: November 26, 2024)

## DISCRIMINATION OF PHASES WITH AVERAGED LOCAL BOND ORDER PARAMETERS

The article presents several snapshots of biased simulations using average local bond order parameters to distinguish liquid phases from crystalline phases. The average local bond order parameters were developed by Lechner and Dellago [1] and are a modification of the so-called local bond order parameters, also called Steinhardt order parameters [2]. Steinhardt order parameters are defined as

$$q_l(i) = \sqrt{\frac{4\pi}{2l+1}\sum_{m=-l}^{l}|q_{lm}(i)|^2}. \tag{1}$$

with

$$q_{lm}(i) = \frac{1}{N_b(i)}\sum_{j=1}^{N_b(i)} Y_{lm}(\mathbf{r}_{ij}). \tag{2}$$

Here $N_b(i)$ is the number of nearest neighbors to atom $i$. $Y_{lm}$ are spherical harmonics with $l$ being the degree and $m$ the order of the spherical harmonic. $\mathbf{r}_{ij}$ is the connecting vector from particle $i$ to particle $j$. The average local bond order parameters are created by introducing an additional averaging of the averaged spherical harmonic contributions to $q_{lm}(i)$ resulting in

$$\bar{q}_l(i) = \sqrt{\frac{4\pi}{2l+1}\sum_{m=-l}^{l}|\bar{q}_{lm}(i)|^2}, \tag{3}$$

with

$$\bar{q}_{lm}(i) = \frac{1}{\tilde{N}_b(i)}\sum_{k=0}^{\tilde{N}_b(i)} q_{lm}(k). \tag{4}$$

where the sum from $k = 0$ to $\tilde{N}_b(i)$ adds up the contribution from all nearest neighbors and the particle itself. $q_{lm}(k)$ is defined by Eq. (2). In the simulation snapshots the average local bond order parameters $\bar{q}_6$ with a 3.5 Å cut off value are calculated for oxygen atoms to distinguish liquid water from hexagonal ice, to distinguish liquid $TiO_2$ from rutile $\bar{q}_8$ are calculated over the 12 nearest neighbors of Ti and to distinguish liquid $TiO_2$ from anatase $\bar{q}_1 0$ are calculated over the 12 nearest neighbor atoms of Ti. The respective thresholds of $\bar{q}_6 = 0.07$ for hexagonal ice, $\bar{q}_8 = 0.073$ for rutile, and $\bar{q}_{10} = 0.085$ for anatase were obtained by visual inspection of the histograms of the average bond order parameters at the beginning (unbiased) and end of the observed crystallization processes triggered by the

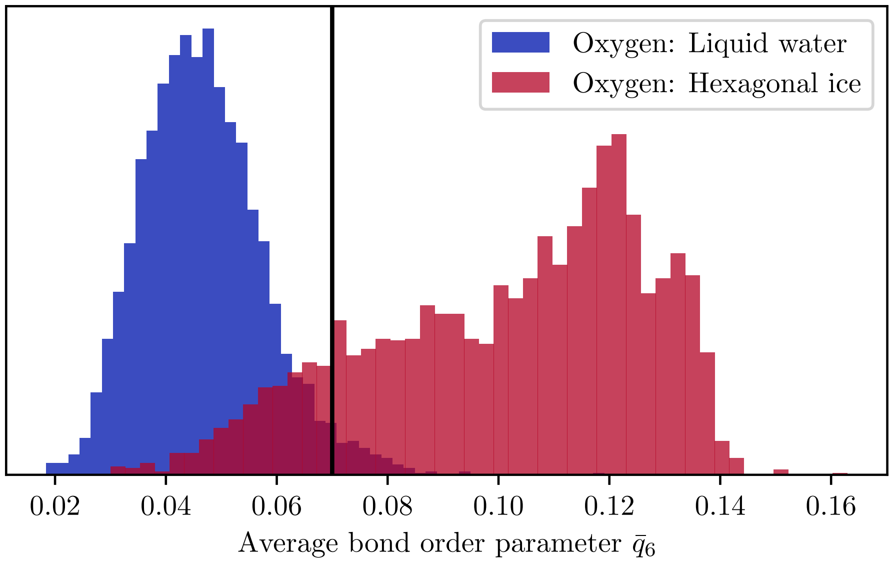


**Figure S1.** Histograms of the average local bond order parameters $\bar{q}_6$ calculated for oxygen atoms in unbiased liquid water (blue) and hexagonal ice created through biasing. The black line marks $\bar{q}_6 = 0.07$.

biased simulations. Figure S1–S3 show the obtained histograms for the simulated transitions from liquid water to hexagonal ice, liquid $TiO_2$ to rutile, and liquid $TiO_2$ to anatase at the start (blue) and end (red) of the biased simulations, respectively. The average local bond order parameters used to distinguish the liquid from the solid phases are marked by the black vertical line.

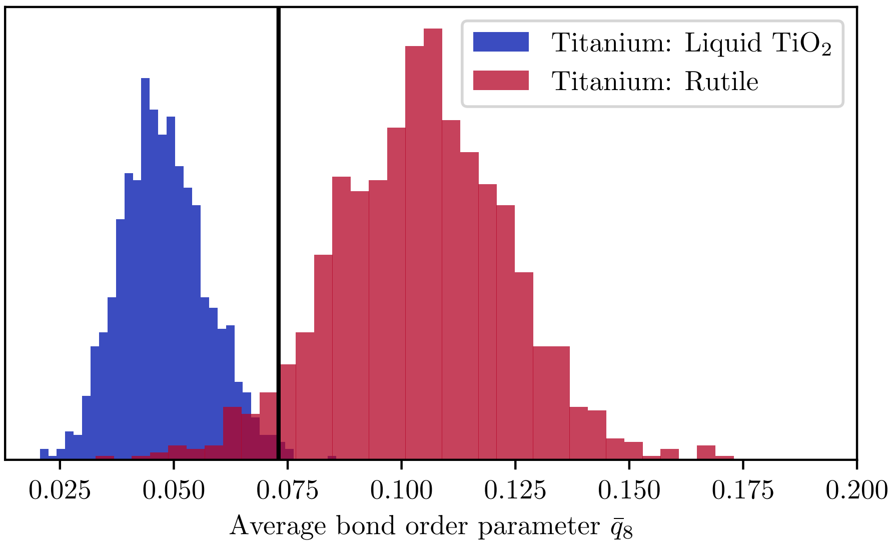


**Figure S2.** Histograms of the average local bond order parameters $\bar{q}_8$ calculated for titanium atoms in unbiased liquid $TiO_2$ (blue) and rutile created through biasing. The black line marks $\bar{q}_8 = 0.073$.

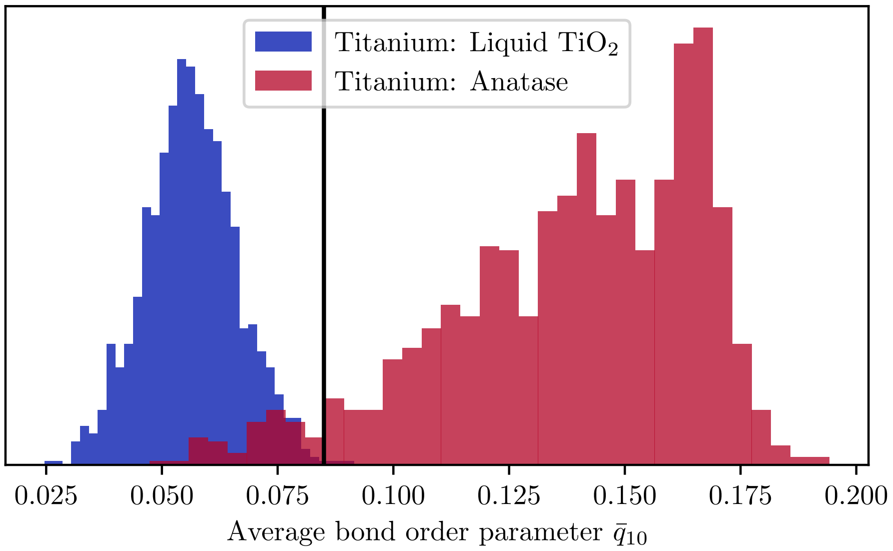


**Figure S3.** Histograms of the average local bond order parameters $\bar{q}_1 0$ calculated for titanium atoms in unbiased liquid $TiO_2$ (blue) and anatase created through biasing. The black line marks $\bar{q}_{10} = 0.085$.

[1] W. Lechner and C. Dellago, Accurate determination of crystal structures based on averaged local bond order parameters, The Journal of Chemical Physics **129**, 114707 (2008).

[2] P. J. Steinhardt, D. R. Nelson, and M. Ronchetti, Bond-orientational order in liquids and glasses, Physical Review B **28**, 784 (1983).
